# Supplementary material for: Gravitational corrections to the two-loop beta function in a non-Abelian gauge theory
Source: arXiv:2408.02512 source file (2024-08-05)
Supplement: Supplementary file 1 [file Einstein_QCD_SM02.pdf]

# Supplemental Material: Gravitational corrections to the two-loop beta function in a non-Abelian gauge theory

M. Gomes,<sup>1,\*</sup> A. C. Lehum,<sup>2,†</sup> and A. J. da Silva<sup>1,‡</sup>

<sup>1</sup>*Instituto de Física, Universidade de São Paulo,*

*Caixa Postal 66318, 05315-970, São Paulo, São Paulo, Brazil.*

<sup>2</sup>*Faculdade de Física, Universidade Federal do Pará, 66075-110, Belém, Pará, Brazil.*

This supplemental material accompanies the paper titled "Gravitational corrections to the two-loop beta function in a non-Abelian gauge theory." In this document, we provide additional information and detailed calculations that were omitted from the main text, including the two-loop diagrams associated with the gluon self-energy. Throughout this supplementary material, we adopt natural units with  $c = \hbar = 1$ , and employ the spacetime signature  $(+ - - -)$ .

## I. GRAVITATIONAL CORRECTIONS TO THE TWO-LOOP GLUON SELF-ENERGY

In this supplementary material, we focus on evaluating the gravitational corrections to the renormalization of the two-loop gluon self-energy. As discussed in the main text, computing this function will suffice to determine the gravitational corrections to the two-loop beta function of the gauge coupling constant. The diagrams contributing to this process are illustrated in Figures 2-4.

Figures 4 depict gravitational corrections involving matter loops. The cumulative effect of these diagrams may contain terms proportional to  $(p^2 \eta^{\mu\nu} - p^\mu p^\nu) \kappa^2 m^2$ , suggesting their renormalization by the constant  $Z_3$ . Our current task in this supplementary material is to provide details omitted in the main text.

To conduct this calculation, we constructed the amplitude using a suite of computational packages [1–5]. In the context of dimensional regularization, among the diagrams in Fig. 4, diagrams 1-2, 16-17, and 19-22 are either null or finite. For the UV divergent diagrams, we have the following expressions:

---

\*Electronic address: mgomes@fma.if.usp.br

†Electronic address: lehum@ufpa.br

‡Electronic address: ajsilva@fma.if.usp.br

$$\begin{aligned}
(\Pi^{\text{ab}})^{\mu\nu}_3(p) &= \frac{i \kappa^2 (p^2 g^{\mu\nu} - p^\mu p^\nu) g_s^2 m_f^2 \delta^{ab}}{12288 \pi^4 \varepsilon^2} - \\
&\frac{i \kappa^2 g_s^2 m_f^2 ((-4 \log(m_f^2) + 4 \log(4\pi) - 4\gamma + 19) p^\mu p^\nu + g^{\mu\nu} ((4 \log(m_f^2) - 4 \log(4\pi) + 4\gamma - 7) p^2 + 54 m_f^2)) \delta^{ab}}{24576 \pi^4 \varepsilon} + O(\varepsilon^0), \\
(\Pi^{\text{ab}})^{\mu\nu}_4(p) &= \frac{i \kappa^2 (p^2 g^{\mu\nu} - p^\mu p^\nu) g_s^2 m_f^2 \delta^{ab}}{12288 \pi^4 \varepsilon^2} - \\
&\frac{i \kappa^2 g_s^2 m_f^2 ((-4 \log(m_f^2) + 4 \log(4\pi) - 4\gamma + 19) p^\mu p^\nu + g^{\mu\nu} ((4 \log(m_f^2) - 4 \log(4\pi) + 4\gamma - 7) p^2 + 54 m_f^2)) \delta^{ab}}{24576 \pi^4 \varepsilon} + O(\varepsilon^0), \\
(\Pi^{\text{ab}})^{\mu\nu}_5(p) &= -\frac{3 i \kappa^2 (p^2 g^{\mu\nu} - p^\mu p^\nu) g_s^2 m_f^2 \delta^{ab}}{1024 \pi^4 \varepsilon} + O(\varepsilon^0), \\
(\Pi^{\text{ab}})^{\mu\nu}_6(p) &= \frac{i \kappa^2 (p^2 g^{\mu\nu} - p^\mu p^\nu) g_s^2 m_f^2 \delta^{ab}}{12288 \pi^4 \varepsilon^2} - \\
&\frac{i \kappa^2 g_s^2 m_f^2 ((-4 \log(m_f^2) + 4 \log(4\pi) - 4\gamma + 19) p^\mu p^\nu + g^{\mu\nu} ((4 \log(m_f^2) - 4 \log(4\pi) + 4\gamma - 7) p^2 + 54 m_f^2)) \delta^{ab}}{24576 \pi^4 \varepsilon} + O(\varepsilon^0), \\
(\Pi^{\text{ab}})^{\mu\nu}_7(p) &= \frac{i \kappa^2 (p^2 g^{\mu\nu} - p^\mu p^\nu) g_s^2 m_f^2 \delta^{ab}}{12288 \pi^4 \varepsilon^2} - \\
&\frac{i \kappa^2 g_s^2 m_f^2 ((-4 \log(m_f^2) + 4 \log(4\pi) - 4\gamma + 19) p^\mu p^\nu + g^{\mu\nu} ((4 \log(m_f^2) - 4 \log(4\pi) + 4\gamma - 7) p^2 + 54 m_f^2)) \delta^{ab}}{24576 \pi^4 \varepsilon} + O(\varepsilon^0), \\
(\Pi^{\text{ab}})^{\mu\nu}_8(p) &= -\frac{3 i \kappa^2 (p^2 g^{\mu\nu} - p^\mu p^\nu) g_s^2 m_f^2 \delta^{ab}}{1024 \pi^4 \varepsilon} + O(\varepsilon^0), \\
(\Pi^{\text{ab}})^{\mu\nu}_9(p) &= \frac{i \kappa^2 (p^2 g^{\mu\nu} - p^\mu p^\nu) g_s^2 m_f^2 \delta^{ab}}{512 \pi^4 \varepsilon^2} + \\
&\frac{i \kappa^2 g_s^2 m_f^2 ((36 \log(m_f^2) - 36 \log(4\pi) + 36\gamma - 23) p^\mu p^\nu + g^{\mu\nu} ((-36 \log(m_f^2) + 36 \log(4\pi) - 36\gamma + 29) p^2 + 27 m_f^2)) \delta^{ab}}{9216 \pi^4 \varepsilon} + O(\varepsilon^0), \\
(\Pi^{\text{ab}})^{\mu\nu}_{10}(p) &= -\frac{i \kappa^2 (p^2 g^{\mu\nu} - p^\mu p^\nu) g_s^2 m_f^2 \delta^{ab}}{1024 \pi^4 \varepsilon^2} + \frac{i \kappa^2 (2 \log(m_f^2) - 2 \log(4\pi) + 2\gamma - 3) (p^2 g^{\mu\nu} - p^\mu p^\nu) g_s^2 m_f^2 \delta^{ab}}{1024 \pi^4 \varepsilon} + O(\varepsilon^0), \\
(\Pi^{\text{ab}})^{\mu\nu}_{11}(p) &= -\frac{i \kappa^2 (p^2 g^{\mu\nu} - p^\mu p^\nu) g_s^2 m_f^2 \delta^{ab}}{1024 \pi^4 \varepsilon^2} + \frac{i \kappa^2 (2 \log(m_f^2) - 2 \log(4\pi) + 2\gamma - 3) (p^2 g^{\mu\nu} - p^\mu p^\nu) g_s^2 m_f^2 \delta^{ab}}{1024 \pi^4 \varepsilon} + O(\varepsilon^0), \\
(\Pi^{\text{ab}})^{\mu\nu}_{12}(p) &= -\frac{i \kappa^2 (p^2 g^{\mu\nu} - p^\mu p^\nu) g_s^2 m_f^2 \delta^{ab}}{1024 \pi^4 \varepsilon^2} + \frac{i \kappa^2 (2 \log(m_f^2) - 2 \log(4\pi) + 2\gamma - 3) (p^2 g^{\mu\nu} - p^\mu p^\nu) g_s^2 m_f^2 \delta^{ab}}{1024 \pi^4 \varepsilon} + O(\varepsilon^0), \\
(\Pi^{\text{ab}})^{\mu\nu}_{13}(p) &= -\frac{i \kappa^2 (p^2 g^{\mu\nu} - p^\mu p^\nu) g_s^2 m_f^2 \delta^{ab}}{1024 \pi^4 \varepsilon^2} + \frac{i \kappa^2 (2 \log(m_f^2) - 2 \log(4\pi) + 2\gamma - 3) (p^2 g^{\mu\nu} - p^\mu p^\nu) g_s^2 m_f^2 \delta^{ab}}{1024 \pi^4 \varepsilon} + O(\varepsilon^0), \\
(\Pi^{\text{ab}})^{\mu\nu}_{14}(p) &= \frac{5 i \kappa^2 (p^2 g^{\mu\nu} - p^\mu p^\nu) g_s^2 m_f^2 \delta^{ab}}{6144 \pi^4 \varepsilon^2} + \\
&\frac{i \kappa^2 g_s^2 m_f^2 ((60 \log(m_f^2) - 60 \log(4\pi) + 60\gamma + 31) p^\mu p^\nu + g^{\mu\nu} (27 m_f^2 - 5 p^2 (12 \log(m_f^2) - 12 \log(4\pi) + 12\gamma + 5))) \delta^{ab}}{36864 \pi^4 \varepsilon} + O(\varepsilon^0), \\
(\Pi^{\text{ab}})^{\mu\nu}_{15}(p) &= \frac{5 i \kappa^2 (p^2 g^{\mu\nu} - p^\mu p^\nu) g_s^2 m_f^2 \delta^{ab}}{6144 \pi^4 \varepsilon^2} + \\
&\frac{i \kappa^2 g_s^2 m_f^2 ((60 \log(m_f^2) - 60 \log(4\pi) + 60\gamma + 31) p^\mu p^\nu + g^{\mu\nu} (27 m_f^2 - 5 p^2 (12 \log(m_f^2) - 12 \log(4\pi) + 12\gamma + 5))) \delta^{ab}}{36864 \pi^4 \varepsilon} + O(\varepsilon^0), \\
(\Pi^{\text{ab}})^{\mu\nu}_{18}(p) &= \frac{3 i \kappa^2 (p^2 g^{\mu\nu} - p^\mu p^\nu) g_s^2 m_f^2 \delta^{ab}}{256 \pi^4 \varepsilon} + O(\varepsilon^0), \\
(\Pi^{\text{ab}})^{\mu\nu}_{23}(p) &= \frac{i \kappa^2 g_s^2 m_f^2 (8 p^\mu p^\nu + g^{\mu\nu} (27 m_f^2 - 2 p^2)) \delta^{ab}}{6144 \pi^4 \varepsilon} + O(\varepsilon^0),
\end{aligned}$$

where we evaluated the integrals retaining only the UV divergent part of  $\Pi(p^2 = 0)$ , as these contributions are only logarithmically divergent. It is important to note that double poles cancel out, while the diagrams with single poles provide the result mentioned in the main text.

## II. FINAL REMARKS

In summary, this supplementary material provides detailed computations of the gravitational corrections to the two-loop self-energy of the gluon field, specifically focusing on contributions from internal matter loops.

## Acknowledgments

A. C. Lehum and A. J. da Silva are partially supported by Conselho Nacional de Desenvolvimento Científico e Tecnológico (CNPq).

- 
- [1] V. Shtabovenko, R. Mertig and F. Orellana, *Comput. Phys. Commun.* **256**, 107478 (2020) doi:10.1016/j.cpc.2020.107478 [arXiv:2001.04407 [hep-ph]].
  - [2] T. Hahn, *Comput. Phys. Commun.* **140**, 418-431 (2001) doi:10.1016/S0010-4655(01)00290-9 [arXiv:hep-ph/0012260 [hep-ph]].
  - [3] A. Alloul, N. D. Christensen, C. Degrande, C. Duhr and B. Fuks, *Comput. Phys. Commun.* **185**, 2250-2300 (2014) doi:10.1016/j.cpc.2014.04.012 [arXiv:1310.1921 [hep-ph]].
  - [4] R. Mertig and R. Scharf, *Comput. Phys. Commun.* **111**, 265-273 (1998) doi:10.1016/S0010-4655(98)00042-3 [arXiv:hep-ph/9801383 [hep-ph]].
  - [5] S. P. Martin and D. G. Robertson, *Comput. Phys. Commun.* **174**, 133-151 (2006) doi:10.1016/j.cpc.2005.08.005 [arXiv:hep-ph/0501132 [hep-ph]].

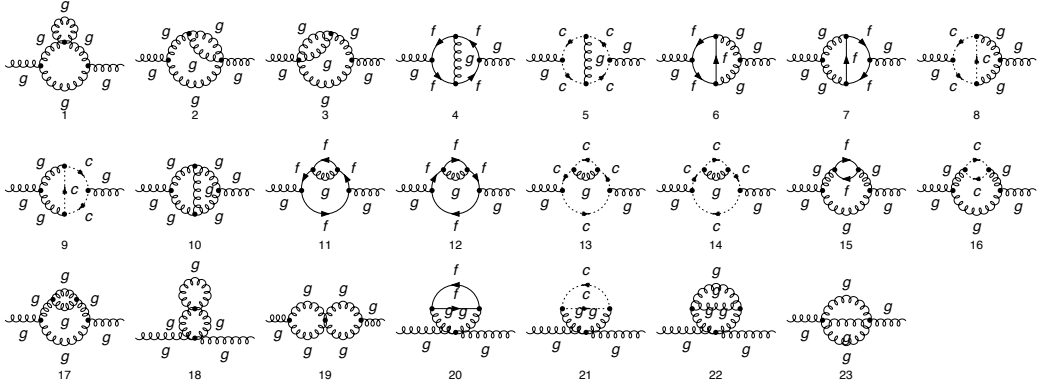

Figure 2: Feynman diagrams depicting the gluon self-energy. Curly and straight lines symbolize the gluon and fermion propagators, respectively.

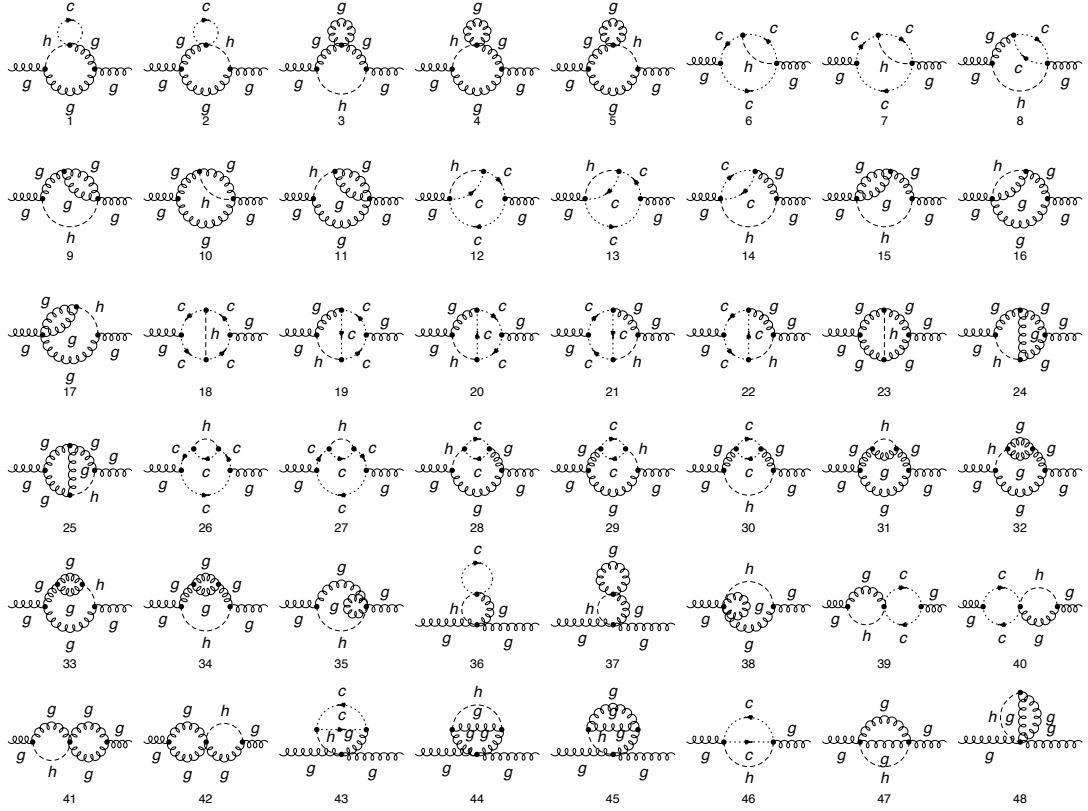

Figure 3: Feynman diagrams illustrating the gluon self-energy incorporating gravitational interaction.

These diagrams consist of terms proportional solely to  $\mathcal{O}(\kappa^2 p^4)$ .

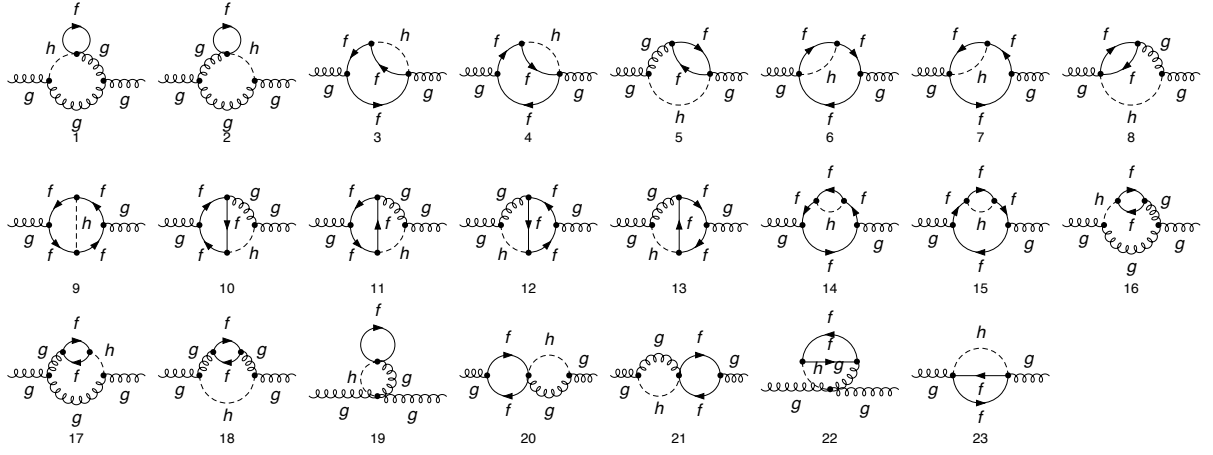

Figure 4: Feynman diagrams depicting the gluon self-energy with contributions from matter and graviton propagators. These diagrams include terms proportional to  $\kappa^2 m^2$  for  $\Pi(p)$ , in addition to  $\kappa^2 p^2$ .
